# Supplementary material for: Zero-phonon line emission of single photon emitters in helium-ion treated MoS$_2$
Source: arXiv:2601.12521 source file (2026-01-18)
Supplement: Supplementary file 2 [file preamble_supplement.tex]

\usepackage{changes}
\usepackage[utf8]{inputenc}
\usepackage{blindtext}
\usepackage{chemformula}
\usepackage[T1]{fontenc}
\usepackage{graphicx}
\usepackage{natbib}
\usepackage{textgreek}
\usepackage{siunitx}
\usepackage[utf8]{inputenc}
\usepackage{amsmath}
\usepackage{xcolor}
\definecolor{fandango}{RGB}{0.71, 0.2, 0.54}
%\usepackage[linkcolor=fandango, colorlinks=true, citecolor=fandango, urlcolor=fandango]{hyperref}
%\usepackage{xr-hyper}
\usepackage{hyperref}
\usepackage[version=4]{mhchem}

%\renewcommand{\figurename}{Fig.}
\renewcommand{\thefigure}{S\arabic{figure}}
\renewcommand{\thepage}{S\arabic{page}}

\setlength\parindent{0pt}

\newcommand{\SIerr}[3]{\SI[separate-uncertainty = true]{#1(#2)}{#3}}
\newcommand{\neutX}{X$^0_\text{1s}$}
\newcommand{\Tbath}{$T_\text{bath}$}
\newcommand{\Pexc}{$P_\text{exc}$}
\newcommand{\Eexc}{$E_\text{exc}$}
\newcommand{\gammahom}{$\gamma_\text{hom}$}
\newcommand{\gammainhom}{$\gamma_\text{inhom}$}
\newcommand{\gzwo}[1][\empty]{%
  g^{(2)}(\tau%
  \ifx#1\empty
    % No 0 provided, so only \tau
  \else
    \!=\!0%
  \fi
  )%
}

\usepackage{xr}

\bibliographystyle{apsrev4-2}
% \externaldocument{main}
